# Supplementary material for: Local Aggregation for Unsupervised Learning of Visual Embeddings
Source: arXiv:1903.12355 source file (2019-04-10)
Supplement: Supplementary file 1 [file analysis_for_supp.tex]

\subsection{Neighbor Identification Procedure Settings}\label{sec:exp_nei}
As mentioned in section~\ref{sec:nei_iden}, we have two candidate procedures for identifying neighbors.
In this subsection, we show empirical evidences and provide some intuitive explanations for specific choices about which procedures to use and also what the parameters of the procedures should be for $\SemNei$ and $\ConNei$.

\begin{table}
\begin{center}
\begin{tabular}{c|c|c|c}
\hline
\diagbox[width=5em]{$\SemNei$}{$\ConNei$} & \thead{Nearest: \\ $\mathcal{N}_{4096}$} & \thead{Clustering: \\ $\mathrm{KM}_{300}$} & $U$ \\
\hline\hline
$\{i\}$ & 33.9 & ?? & ??  \\
\hline
\thead{Nearest: \\ $\mathcal{N}_{\{2, 5, 10, 20, 100, 200\}}$} & \texttt{NT} & \texttt{NT} & \texttt{NT}  \\
\hline
\thead{Clustering: \\ $\mathrm{KM}_{10000}$} & \textbf{35.7} & 33.2 & 30.2  \\
\hline
\end{tabular}
\end{center}
\caption{
Best validation performances in percentages for networks trained with different neighbor identification procedures for semantic and context neighbors.
\texttt{NT} means the model is \textbf{NOT} trainable under that setting.
$U$ represents $\{1, 2, ..., N\}$.
$\mathrm{KM}_k$ means the clustering results by KMeans algorithm with $k$ clusters.
}
\label{tab:nei}
\end{table}

\textbf{Procedure combination search}.
To find the empirically best neighbor identification procedure combination, we vary the choices for $\SemNei$ and $\ConNei$ and then train a ResNet-18 model on ImageNet.
Besides the nearest-neighbor based identification and the clustering based identification, we also include additional trivial options: $\{i\}$ for $\SemNei$ and $U = \{1, 2, ..., N\}$ for $\ConNei$.
Meanwhile, we assume that the performance gains from the changing the parameters within procedure, such as $k$ in $\mathcal{N}_k$, are independent of the gains from the procedure choices.
With this assumption, we can then postpone the fine-tuning of parameters within the procedures until a combination choice has been made.
After training networks with different combination choices, we then report their best validation performances in Table~\ref{tab:nei}.
The detailed explanations about these results are provided below:
\begin{enumerate}
  \item 
  We use KMeans~\cite{lloyd1982least} with 10000 clusters for clustering based method of $\SemNei$. 
  As mentioned in section~\ref{sec:mem_bank}, KMeans is applied to the memory bank to get the cluster assignments.
  To achieve a balance between performances and efficiency, we update the KMeans result at the end of every epoch.
  Although this updating frequency, the number of clusters, and even the clustering algorithm can vary, we delay the explorations on these parameters until completing this combination search.
  Similarly, we use $\mathcal{N}_{4096}$ for nearest neighbor based method of $\ConNei$.
  Moreover, we use KMeans with 300 clusters for clustering based method of $\ConNei$ to achieve a similar number of neighbors to $\mathcasl{N}_{4096}$, as each cluster in KMeans results will roughly have $1.2\mathrm{M} / 300 = 4000$ images.
  \item 
  We find that the models using nearest neighbors $\mathcal{N}_k$ as $\SemNei$ all fail to give any non-trivial performances, regardless of the procedures chosen for $\ConNei$.
  To ensure that this failure is also independent of the parameter choice in building the nearest neighbors for $\SemNei$, we vary the $k$ in $\mathcal{N}_k$ from 2 to 200 and show that the models are still \textbf{NOT} trainable.
  \textcolor{red}{[TODO: Add a figure intuitively explaining that this might be related to density biases nearest neighbor can introduce.]}
  \item 
  We find that a local context is useful, which can be shown through the improvements of performances after changing $\ConNei$ from $U$ to local neighbors.
  We hypothesize that the large number of neighbors in $\ConNei$ makes the gradients from $\SemNei^c \cap \ConNei$ significantly bigger than the gradients from $\SemNei \cap \ConNei$.
  Instead, a local context can balance these gradients.
  \item
  Nearest neighbors are better $\ConNei$ than clustering based neighbors, as shown by the differences between the columns with $\ConNei = \mathcal{N}_{4096}$ and the columns with KMeans results as $\ConNei$.
  We believe this is due to the fact that nearest neighbors $\mathcal{N}_k(\VI)$ are dependent on $\VI$ and therefore more dynamic than clustering results, which are based on the memory bank.
  \item
  Overall, the model using KMeans results as $\SemNei$ and $\mathcal{N}_{4096}$ as $\ConNei$ achieves the best validation performance in Table~\ref{tab:nei}. 
  
\end{enumerate}

\textbf{Clustering algorithm}.
Given that the best model involves clustering algorithms, we next consider whether our current choice, KMeans, is the best one. 
Despite the variety of unsupervised clustering algorithms such as KMeans, DBSCAN~\cite{ester1996density}, and Affinity Propagation~\cite{frey2007clustering}, most of them are \textbf{NOT} scalable to large-scale datasets, which greatly limits our choices.
In consequence, only KMeans and DBSCAN are applicable to our problem of clustering million examples within a reasonable time.
Among these two algorithms, DBSCAN is known to perform worse in higher dimension data and varying density space~\cite{ester1996density}.
Unfortunately, the embedding space we are working with has both these two features.
Indeed, we find that when applied to the memory bank, DBSCAN always gives trivial results, regardless of how we vary the adjustable parameters (see Supplementary for details). 
Therefore, KMeans is actually our only choice.
Following~\cite{caron2018deep}, we use Faiss~\cite{JDH17} which can efficiently cluster large-scale datasets.

\textbf{Combining multiple cluster assignments}.
As mentioned in section~\ref{sec:nei_iden}, we can combine multiple clustering results as neighbors using either intersection ($\bigcap$) or union ($\bigcup$) operations.
More specifically, assuming that we apply KMeans $H$ times to $\MemBank$ with different $k$s or the same $k$s but different initializations so that we have $H$ cluster results $\{ \mathbf{G}^{(j)} \}$ with their label functions $\{g^{(j)}\}$, we can then use $\bigcup_{j=1}^{H} G_{g^{(j)}(\VI)}^{(j)}$ or $\bigcap_{j=1}^{H} G_{g^{(j)}(\VI)}^{(j)}$ as the neighbors of $\VI$.
We denote this procedure as $\bigcup_{j=1}^H \mathrm{KM}_{k_j}$ or $\bigcap_{j=1}^H \mathrm{KM}_{k_j}$.
Moreover, if the $k$s are all the same, we further simplify the notations as $\bigcup^H \mathrm{KM}_k$ or $\bigcap^H \mathrm{KM}_k$.
In order to find the optimal settings, we train the networks with different $H$ and $k$s. 
The performances of these networks are shown in Table~\ref{tab:combine}.
%let $\mathrm{KM}_k$ be the KMeans result with $k$ clusters, we then use $\bigcup^H \mathrm{KM}_k$ to represent the method of identifying neighbors for $\VI$ through combining $H$ clusters 
%In fact, we find that the combinations with $\bigcup$ lead to significantly better results.
We summarize our findings below:
\begin{enumerate}
  \item 
  For networks using single KMeans result, varying parameter $k$ slightly influences the model performances, while $10000$ seems to be the optimal value, at least for structure ResNet-18.
  This conclusion can be drawn through comparing the performances of ResNet-18 with $\mathrm{KM}_{1000}$, $\mathrm{KM}_{10000}$, and $\mathrm{KM}_{20000}$.
  \item
  Combining multiple KMeans results with unions works better than single result, while combining with intersections hurts the performance. 
  This can be shown through comparing ResNet-18 performances trained with $\bigcup^3 \mathrm{KM}_{10000}$, $\mathrm{KM}_{10000}$, and $\bigcap^3 \mathrm{KM}_{10000}$. 
  We hypothesize that this performance difference is because the unions of multiple results as $\SemNei$ will be more likely to center around $\VI$, while single result and intersections might have $\VI$ close to the boundary, which makes $\SemNei$ a worse set of neighbors.
  To intuitively illustrate this hypothesis, we show some examples for unions and intersections of multiple results in Figure~\ref{fig:clster}.
  \item
  The optimal parameter pair $(H, k)$ are dependent on the network architecture. 
  For example, AlexNet reaches its best performance for $(3, 10000)$, while $(10, 30000)$ is optimal for both ResNet-18 and ResNet-50.
  We believe this dependence can be explained through recognizing the fact that deeper architecture has more semantically similar neighbors, as shown by its higher validation performance.
  Moreover, unions of more results can not only include more neighbors, but also make the neighbors more centered, as shown in Figure~\ref{fig:clster}.
  Therefore, bigger set of neighbors can help more in deeper network, while in shallower network, bigger set may even hurt the performance because of including neighbors of low similarity.
  This explanation can also be supported by the performance \textbf{drop} for AlexNet from $(3, 10000)$ to $(6, 10000)$, which includes more neighbors, despite the performance \textbf{gain} for ResNet-18 with the same parameter change.
  Additionally, the \textbf{big} performance drop for ResNet-18 from $(6, 10000)$ to $(10, 10000)$ and the \textbf{slight} performance performance change for ResNet-50 with the same parameter change are also consistent with our explanation.
  Furthermore, the performance gains for both ResNet-18 and ResNet-50 from $(10, 10000)$ to $(10, 30000)$, which reduces the number of neighbors, means that there exists an optimal neighbor size regarding performances.
  Although from the results we have shown, ResNet-18 and ResNet-50 seem to share the same optimal neighbor size, it is possibly due to the lack of parameter explorations for ResNet-50.
  \item
  Moreover, the performance gain from the optimal pair compared to single KMeans result are also dependent on the network architecture.
  Specifically, the gain for AlexNet is only $0.5\%$, while that for ResNet-18 reaches $2.2\%$ and that for ResNet-50 becomes even bigger: $3.2\%$.
  This gain change across architectures also holds true after considering relative gains instead of absolute gains.
  These results suggest that deeper architectures can benefit more from unions of multiple KMeans results.
  
\end{enumerate}

\begin{table}
\begin{center}
\begin{tabular}{c|ccc}
\hline
\diagbox[width=7em]{Setting}{Network} & AlexNet & ResNet-18 & ResNet-50 \\
\hline\hline
\\[-1em]
$\bigcap^3 \mathrm{KM}_{10000}$ & -- & 34.3 & -- \\ 
\hline
$\mathrm{KM}_{1000}$ & -- & 35.2 & -- \\
\hline
$\mathrm{KM}_{10000}$ & 30.6 & 35.7 & 40.2 \\
\hline
$\mathrm{KM}_{20000}$ & -- & 35.0 & -- \\
\hline
\\[-1em]
$\bigcup^3 \mathrm{KM}_{10000}$ & \textbf{31.1} & 36.2 & --\\
\hline
\\[-1em]
$\bigcup^6 \mathrm{KM}_{10000}$ & 30.4 & 37.3 & 42.4 \\
\hline
\\[-1em]
$\bigcup^{10} \mathrm{KM}_{10000}$ & -- & 36.2 & 42.3 \\
\hline
\\[-1em]
$\bigcup^{10} \mathrm{KM}_{30000}$ & -- & \textbf{37.9} & \textbf{43.4} \\
\hline
\end{tabular}
\end{center}
\caption{
Best validation performances in percentages for networks trained with different combination operations and parameters.
Numbers in bold are the best performances in columns.
}
\label{tab:combine}
\end{table}

\textbf{Other hyper-parameters}.
There are many other adjustable hyper-parameters related to the neighbor identification procedures, such as the updating frequency for the KMeans results, the parameter $k$ in $\mathcal{N}_k$ for $\ConNei$, and whether doing KMeans on $\MemBank$ or network outputs on center crops of $\mathbf{I}$. 
Although it is impossible to exhaust all combinations for these hyper-parameters, we try our best to explore their influences on performances through training ResNet-18 networks with different parameters.
Due to the space limit, we put the details of the training in the supplementary material but summarize our findings below:
\begin{enumerate}
  \item 
  Updating the KMeans results more frequently than every epoch has little influence on performances. Therefore, we choose updating frequency to be every epoch.
  \item
  Varying parameter $k$ in $\mathcal{N}_k$ for $\ConNei$ also influences little on performances. So we continue to use $4096$.
  \item
  Doing KMeans on center crops performs similar to KMeans on $\MemBank$, despite its additional time consumption for getting network outputs on these center crops.
\end{enumerate}
